# Supplementary material for: Unrolled Optimization with Deep Priors
Source: arXiv:1705.08041 ancillary file (2018-12-18)
Supplement: Supplementary file 1 [file supplement.pdf]

---

# Supplementary Information: Unrolled Optimization with Deep Priors

---

Steven Diamond

Vincent Sitzmann

Felix Heide

Gordon Wetzstein

The supplement contains additional supporting material for our submission. In Sec. 1, we present all the ODP networks in detail. In Sec. 2, we give the full details of the training procedure for all the networks presented in the submission and show convergence plots. In Sec. 3, we discuss additional images output by the ODP networks. We used TensorFlow to train and evaluate our models. We will publish all code and trained models upon acceptance.

## 1 Additional Unrolled Optimization Networks

In our submission, we compared ODP networks for proximal gradient, ADMM, LADMM, and gradient descent. We only presented the details of the proximal gradient network in the paper, so we present all the networks in detail here. Algorithm 1 shows a generic ODP proximal gradient network. Algorithm 2 shows a generic ODP ADMM network. Algorithm 3 shows a generic ODP LADMM network. Algorithm 4 shows a generic ODP gradient descent network.

We now present the explicit ODP proximal gradient networks for each application: denoising in Algorithm 5, deblurring in Algorithm 6, and CS MRI in Algorithm 7.

## 2 Network Training Details

In this section we give the full details of the network training for every experimental result presented in the submission.

**CNN prior details** Here we give the full details of the CNN prior proximal operator. We used a single residual connection between input and output, *i.e.*, the output  $x^{k+1/2}$  of the CNN was given by  $x^{k+1/2} = x^k + \phi(x^k)$ , where  $\phi$  is an  $n$ -layer convolutional network with batch normalization and ReLU nonlinearities. The first convolutional layer had 1 or 3 input channels (depending on whether the images were grayscale or color) and  $d$  output channels. The  $n - 2$  intermediate convolutional layers had  $d$  input channels and  $d$  output channels. The final convolutional layer had  $d$  input channels and 1 or 3 output channels (again depending on the number of channels in the image). We used  $d = 64$  for all experiments and  $3 \times 3$  kernels.

**Denoising on noise level  $\sigma = 25$  and test set from [7]** We trained an ODP proximal gradient network for denoising with 4 iterations and a 10 layer, 64 channel residual CNN prior with ReLU nonlinearities. We trained on the 400 image test set from [7], with data augmentation via flipping, rotation by 90 degrees, and dynamic noise generation. We used Xavier initialization [3] for the CNN and parameterized  $\alpha_k$  as  $\alpha_k = C_0 C_k$  with  $C_0$  and  $C_k$  learnable, initialized to  $C_0 = 0$  and  $C_k = 2^{-k}$ . We used a mean-squared-error loss. We used a validation set of 500 images from the ImageNet validation set [2]. We scaled the input images from  $[0, 255]$  and cropped them to  $180 \times 180$ . We used Adam [4] with a learning rate of 0.001 decayed exponentially by factor 0.5 every 300 epochs. We used Adam  $\beta_1 = 0.9$ , Adam  $\beta_2 = 0.999$ , and weight decay 0.0001. We tested the model trained for 134,068 iterations with batch size 4 on a Titan X GPU, chosen through evaluation on the validation set. Figure 1 shows the loss curve (in PSNR dB).

---

**Algorithm 1** ODP proximal gradient network

---

1: Initialization:  $x^0 = \phi(f, A, y, \theta^0)$ ,  $\alpha_k = C_0 C^{-k}$ ,  $C_0 > 0$ ,  $C > 0$   
2: **for**  $k = 0$  to  $N - 1$  **do**  
3:    $x^{k+1/2} \leftarrow \text{CNN}(x^k, \theta^k)$ .  
4:    $x^{k+1} \leftarrow \text{argmin}_x \alpha_k f(Ax, y) + \frac{1}{2} \|x - x^k - x^{k+1/2}\|_2^2$ .  
5: **end for**

---

---

**Algorithm 2** ODP ADMM network

---

1: Initialization:  $(x^0, z^0) = \phi(f, A, y, \theta^0)$ ,  $\rho_k = C_0 C^k$ ,  $C_0 > 0$ ,  $C > 0$   
2: **for**  $k = 0$  to  $N - 1$  **do**  
3:    $x^{k+1/2} \leftarrow \text{CNN}(x^k - z^k, \theta^k)$ .  
4:    $x^{k+1} \leftarrow \text{argmin}_x f(Ax, y) + \frac{\rho_k}{2} \|x - x^{k+1/2} - z^k\|_2^2$ .  
5:    $z^{k+1} \leftarrow z^k + x^{k+1/2} - x^{k+1}$   
6: **end for**

---

---

**Algorithm 3** ODP LADMM network

---

1: Initialization:  $(x^0, z^0, u^0) = \phi(f, A, y, \theta^0)$ ,  $\mu_0, \dots, \mu_{N-1} \geq 0$ ,  $\rho_0, \dots, \rho_{N-1} \geq 0$   
2: **for**  $k = 0$  to  $N - 1$  **do**  
3:    $x^{k+1} \leftarrow \text{CNN}(x^k - (\mu_k / \rho_k) A^H (Ax^k - z^k + u^k), \theta^k)$ .  
4:    $z^{k+1} \leftarrow \text{argmin}_x \rho_k f(Ax, y) + \frac{1}{2} \|x - Ax^{k+1} - u^k\|_2^2$ .  
5:    $u^{k+1} \leftarrow u^k + Ax^{k+1} - z^{k+1}$ .  
6: **end for**

---

---

**Algorithm 4** ODP gradient descent network

---

1: Initialization:  $x^0 = \phi(f, A, y, \theta^0)$ ,  $\alpha_0, \dots, \alpha_{N-1} \geq 0$   
2: **for**  $k = 0$  to  $N - 1$  **do**  
3:    $x^{k+1/2} \leftarrow \text{CNN}(x^k, \theta^k)$ .  
4:    $x^{k+1} \leftarrow x^k - \alpha_k A^T \nabla_x f(Ax^k, y) - x^{k+1/2}$ .  
5: **end for**

---

---

**Algorithm 5** ODP proximal gradient denoising network

---

1: Initialization:  $x^0 = y$ ,  $\alpha_k = C^{-k}$ ,  $C_0 > 0$ ,  $C > 0$   
2: **for**  $k = 0$  to  $N - 1$  **do**  
3:    $x^{k+1/2} \leftarrow \text{CNN}(x^k, \theta^k)$ .  
4:    $x^{k+1} \leftarrow (\alpha_k y + x^k + x^{k+1/2}) / (\alpha_k + 1)$ .  
5: **end for**

---

---

**Algorithm 6** ODP proximal gradient deblurring network.  $\mathcal{F}$  is the DFT,  $k$  is the blur kernel, and  $\mathbf{K}$  is the DFT of  $k$ 

---

1: Initialization:  $x^0 = k^T * y$ ,  $\alpha_k = C^{-k}$ ,  $C_0 > 0$ ,  $C > 0$   
2: **for**  $k = 0$  to  $N - 1$  **do**  
3:    $x^{k+1/2} \leftarrow \text{CNN}(x^k, \theta^k)$ .  
4:    $x^{k+1} \leftarrow \mathcal{F}^{-1} \text{diag}(\alpha_k |\mathbf{K}|^2 + 1)^{-1} \mathcal{F}(\alpha_k k^T * y + x^k + x^{k+1/2})$ .  
5: **end for**

---

**Deblurring using image formation and test set from [8]** We trained an ODP proximal gradient network for deblurring with 8 iterations and a 5 layer, 64 channel residual CNN prior with ReLu nonlinearities. We trained one model for the disk blur kernel and another model for the motion blur kernel on the 1.2e6 ImageNet training images [2], with data augmentation via flipping, rotation by 90 degrees, and dynamic noise generation at  $\sigma = 5.7020$ . We used Xavier initialization [3] for the CNN and parameterized  $\alpha_k$  as  $\alpha_k = C_0 C_k$  with  $C_0$  and  $C_k$  learnable, initialized to  $C_0 = 1000$  and  $C_k = 2^{-k}$ . We used a mean-squared-error loss. Xu et al. also train one model per kernel [8]. We

---

**Algorithm 7** ODP proximal gradient CS MRI network.  $\mathcal{F}$  is the DFT and  $P$  is the binary, diagonal subsampling matrix.

---

```

1: Initialization:  $x^0 = \mathcal{F}^{-1}Py$ 
2: for  $k = 0$  to  $N - 1$  do
3:    $x^{k+1/2} \leftarrow \text{CNN}(\text{Re}(x^k), \theta^k)$ .
4:    $z^{k+1} \leftarrow \mathcal{F}(x^k + x^{k+1/2})$ .
5:    $x^{k+1} \leftarrow \mathcal{F}^{-1}(Py + (I - P)z^{k+1})$ .
6: end for

```

---

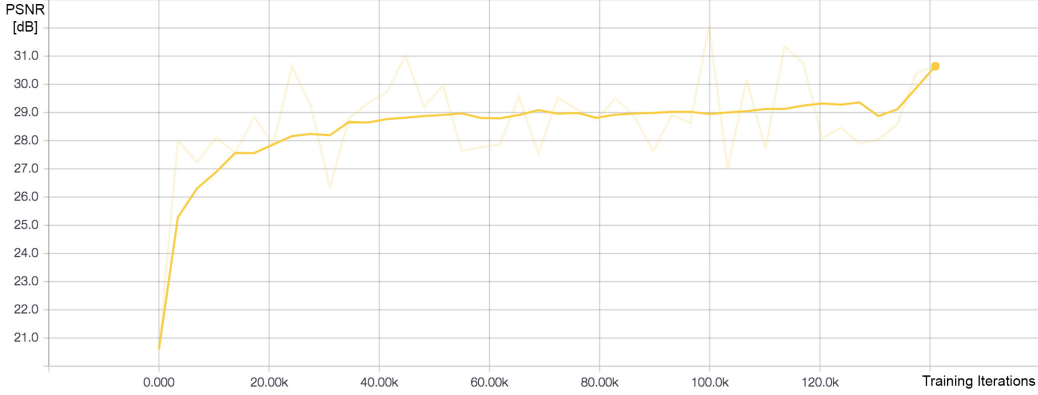

Figure 1: Loss curve in average PSNR (dB) for denoising network

used a validation set of 500 images from the ImageNet validation set [2]. We scaled the input images from  $[0, 255]$  and cropped them to  $256 \times 256$ , with replication padding equal to  $1/2$  the kernel size. Xu et al. used the same padding scheme [8]. We used Adam [4] with a learning rate of 0.01 decayed exponentially by factor 0.5 every 0.25 epochs. We used Adam  $\beta_1 = 0.9$ , Adam  $\beta_2 = 0.999$ , and weight decay 0.0001. We tested the disk blur model trained for 149,820 iterations with batch size 4 on a Titan X GPU, chosen through evaluation on the validation set. We tested the disk blur model trained for 151,736 iterations with batch size 4 on a Titan X GPU, chosen through evaluation on the validation set. Figure 2 shows the loss curve (in PSNR dB).

**Deblurring using image formation and test set from [6]** We trained an ODP proximal gradient network for deblurring with 8 iterations and a 5 layer, 64 channel residual CNN prior with ReLu nonlinearities. We trained one model on the 4 low-pass kernels and another model on 10,000 randomly

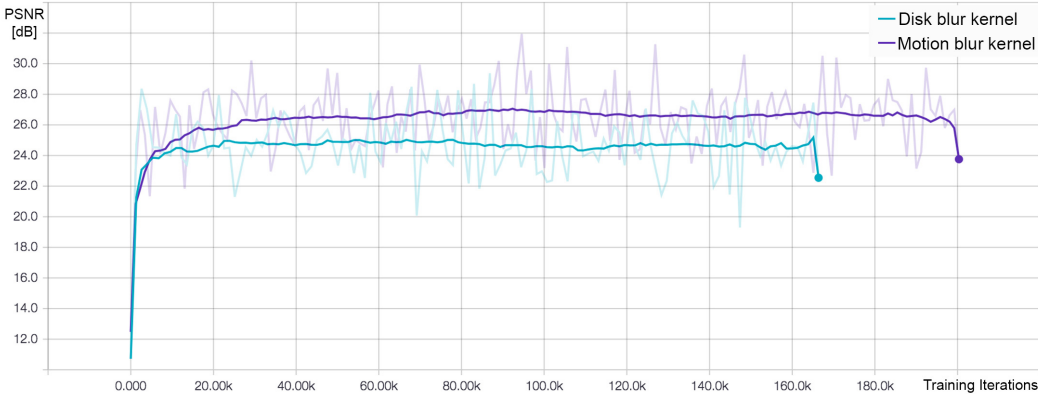

Figure 2: Loss curve in average PSNR (dB) for deblurring networks on disk and motion blur kernels for image formation from [8]

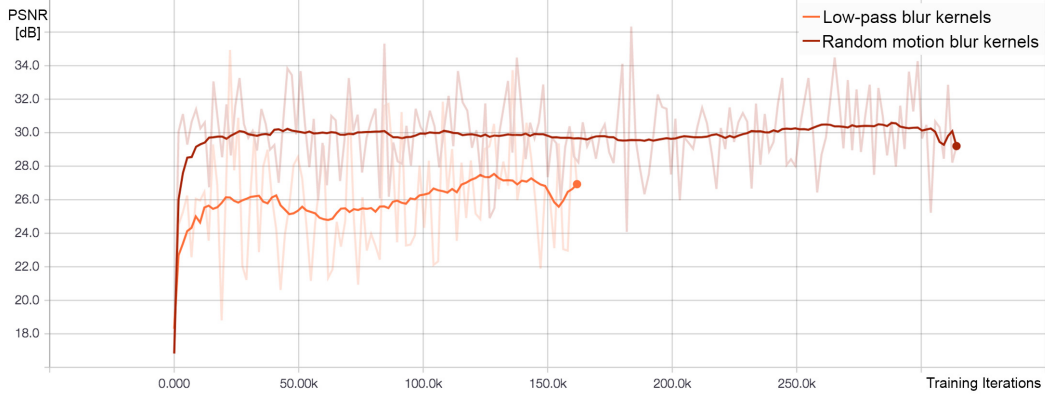

Figure 3: Loss curve in average PSNR (dB) for deblurring networks on low-pass and randomly generated motion blur kernels for image formation from [6]

generated motion blur kernels on the  $1.2e6$  ImageNet training images (the same training data as [6]), with data augmentation via flipping, rotation by 90 degrees, and dynamic noise generation. We used Xavier initialization [3] for the CNN and parameterized  $\alpha_k$  as  $\alpha_k = C_0 C_k$  with  $C_0$  and  $C_k$  learnable, initialized to  $C_0 = 1000$  and  $C_k = 2^{-k}$ . We used a mean-squared-error loss. We generated the random motion blur kernels using the approach in [5]. Schuler et al. train one model per kernel [6]. We used a validation set of 500 images from the ImageNet validation set [2]. We scaled the input images from  $[0, 255]$  and cropped them to  $256 \times 256$ . We followed [6] and did not pad but cropped  $1/2$  the kernel size when evaluating. We used Adam [4] with a learning rate of 0.01 decayed exponentially by factor 0.5 every 0.25 epochs. We used Adam  $\beta_1 = 0.9$ , Adam  $\beta_2 = 0.999$ , and weight decay 0.0001. We tested the low-pass blur model trained for 148,981 iterations with batch size 4 on a Titan X GPU, chosen through evaluation on the validation set. We tested the motion blur model trained for 160,549 iterations with batch size 4 on a Titan X GPU, chosen through evaluation on the validation set. Figure 3 shows the loss curve (in PSNR dB).

**CS MRI using image formation and test set from [9]** We trained an 8 iteration proximal gradient ODP network with a residual 7 layer, 64 channel CNN prior on the same 100 training images of brain MRIs as [9] and evaluated the network on the same 50 test images. We used Xavier initialization [3] for the CNN. We used a mean-squared-error loss. We used the same four pseudo-radial sampling patterns as [9], which range from sampling 20% to 50% of the Fourier domain. We augmented the training data with arbitrary rotations and reflections and used early stopping with a 420 image validation set from [1]. We trained a single model for all four sampling patterns, while Yang et al. trained a separate ADMM-Net model for each pattern. We used Adam [4] with a learning rate of 0.005 decayed exponentially by factor 0.5 every 1000 epochs. We used Adam  $\beta_1 = 0.9$ , Adam  $\beta_2 = 0.999$ , and weight decay 0.0001. We tested the low-pass blur model trained for 102,249 iterations with batch size 8 on a Titan X GPU, chosen through evaluation on the validation set. Figure 4 shows the loss curve (in PSNR dB).

**Proximal gradient networks versus prior-only networks** For the ablation study in which we removed the data step from the ODP proximal gradient networks and evaluated the performance of the resulting residual networks, we used exactly the same training procedure as described above. The prior-only (residual) networks were trained in exactly the same manner as the proximal gradient networks, with convergence determined using the relevant validation set. Figure 5 shows the loss curves in average PSNR dB for the proximal gradient and prior-only denoising networks. Figure 5 shows the loss curves in average PSNR dB for the proximal gradient and prior-only motion deblurring networks.

**Algorithm comparison** For the comparison of the proximal gradient, ADMM, LADMM, and gradient descent algorithms, we used exactly the same training procedure as described above. All networks were trained in exactly the same manner as the proximal gradient networks, with convergence determined using the relevant validation set. For ADMM networks,  $\rho_k$  was parameterized

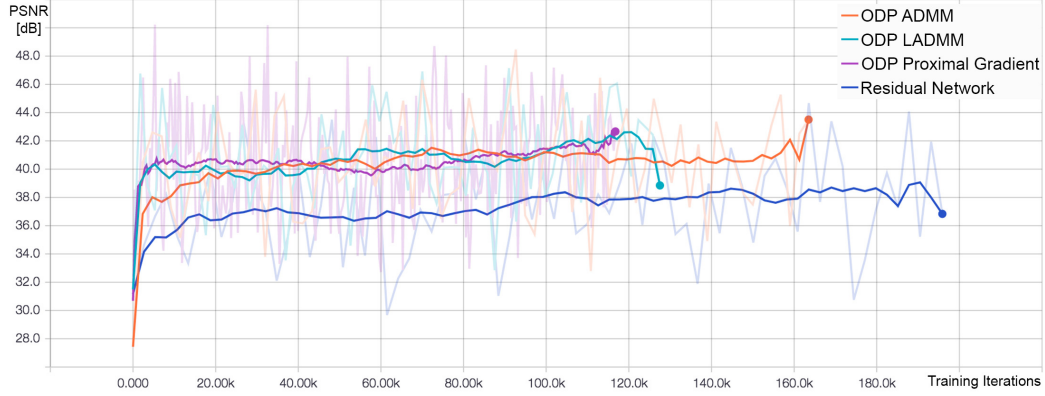

Figure 4: Loss curve in average PSNR (dB) for CS MRI proximal gradient, ADMM, LADMM, and prior only (*i.e.*, residual) networks with image formation from [9]

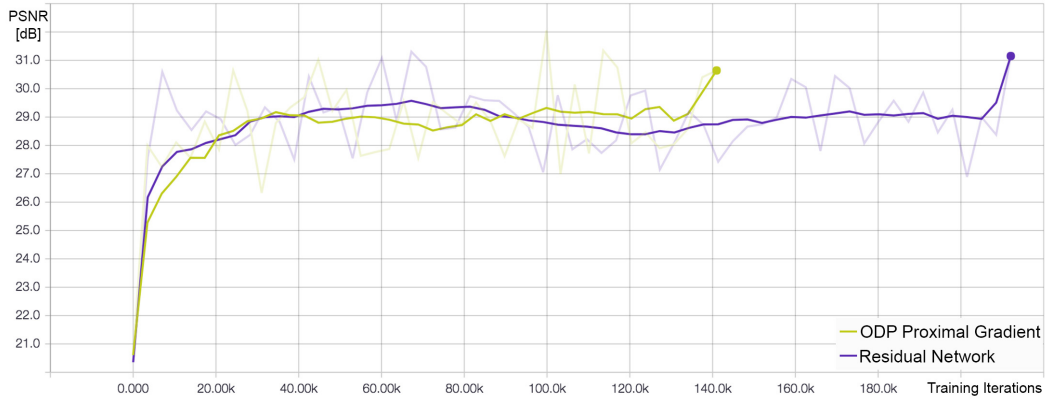

Figure 5: Loss curve in average PSNR (dB) for denoising proximal gradient and prior only (*i.e.*, residual) networks with image formation and noise level from [7]

as  $\rho_k = C_0 C_k$  with  $C_0$  and  $C_k$  learnable, initialized to  $C_0 = 1000$  and  $C_k = 2^k$ . For LADMM networks,  $\mu_k$  and  $\rho_k$  were learned with initialization  $\rho_k = \mu_k = 1$ . For gradient descent networks,  $\alpha_k$  were learned with initialization  $\alpha_k = 0$ . Figure 6 shows the loss curves in average PSNR dB for the proximal gradient, ADMM, LADMM, and gradient descent motion deblurring networks. Figure 4 shows the loss curves in average PSNR dB for the proximal gradient, ADMM, and LADMM CS MRI networks.

### 3 Extended Qualitative Results

We have provided full validation sets for all denoising, deconvolution and CS-MRI experiments as a supplementary archive. The image files with filename suffixes `gt` and `inp` denote the original ground truth image, and the observation according to image formation model from Sections 5.1, 5.2 and 5.3 from the main draft, respectively. The filename suffixes `out` indicate the output of the proximal gradient ODP architecture with the observation `inp` as input. For all considered inverse problem settings, the reconstructions are of high perceptual quality. Only very fine detail in the reconstruction is in some instances lost in the reconstructions, visible in images of fur for denoising, and hair for motion, for instance. This behavior is a result of the mean-squared-error loss and alternating prior/data projection steps in the ODP architecture and is, in fact, desired for inverse problems in sensing and scientific imaging, as hallucinating image features is problematic for diagnostic purposes. Note that an interesting direction for future work is training ODPs using adversarial losses and residual connections in the data step, which could then force ODPs to hallucinate such detail for generative applications with non-diagnostic components, *e.g.*, in graphics.

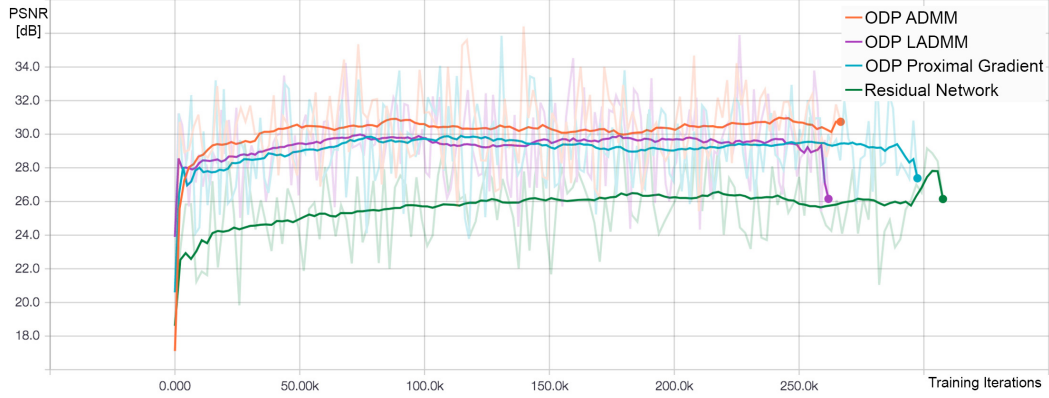

Figure 6: Loss curve in average PSNR (dB) for motion deblurring proximal gradient, ADMM, LADMM, and prior only (*i.e.*, residual) networks with image formation from [6]

## References

- [1] A. Asman, A. Akhondi-Asl, H. Wang, N. Tustison, B. Avants, and S. Warfield. MICCAI 2013 segmentation algorithms, theory and applications (SATA) challenge results summary. In *MICCAI challenge workshop on segmentation: algorithms, theory and applications (SATA)*. 2013.
- [2] Jia Deng, Wei Dong, Richard Socher, Li-Jia Li, Kai Li, and Li Fei-Fei. Imagenet: A large-scale hierarchical image database. In *Computer Vision and Pattern Recognition, 2009. CVPR 2009. IEEE Conference on*, pages 248–255. IEEE, 2009.
- [3] X. Glorot and Y. Bengio. Understanding the difficulty of training deep feedforward neural networks. In *Proceedings of the International Conference on Artificial Intelligence and Statistics*, volume 9, pages 249–256, 2010.
- [4] D. Kingma and J. Ba. Adam: A method for stochastic optimization. *arXiv preprint arXiv:1412.6980*, 2014.
- [5] U. Schmidt and S. Roth. Shrinkage fields for effective image restoration. In *Proceedings of the IEEE Conference on Computer Vision and Pattern Recognition*, pages 2774–2781, 2014.
- [6] C. Schuler, H. Burger, S. Harmeling, and B. Scholkopf. A machine learning approach for non-blind image deconvolution. In *Proceedings of the IEEE Conference on Computer Vision and Pattern Recognition*, pages 1067–1074, 2013.
- [7] S. Wang, S. Fidler, and R. Urtasun. Proximal deep structured models. In *Advances in Neural Information Processing Systems 29*, pages 865–873. 2016.
- [8] L. Xu, J. Ren, C. Liu, and J. Jia. Deep convolutional neural network for image deconvolution. In *Advances in Neural Information Processing Systems*, pages 1790–1798, 2014.
- [9] Y. Yang, J. Sun, H. Li, and Z. Xu. Deep ADMM-Net for compressive sensing MRI. In *Advances in Neural Information Processing Systems*, pages 10–18, 2016.
